# Supplementary material for: NNLO anomalous dimension matrix for twist-two flavor-singlet operators
Source: arXiv:2205.08228 ancillary file (2022-05-17)
Supplement: Supplementary file 1 [file README.pdf]

Files `Anc1.mres` and `Anc2.mres` contain the MATHEMATICA versions of the results given in a shortened form in Section 4 of V.M. Braun, K.G. Chetyrkin and A.N. Manashov “NNLO anomalous dimension matrix for twist-two flavor-singlet operators”.

Notations:

`z3`, `z4`, `z5` stand for the values of the Riemann zeta-function with  $z3 = \zeta_3 = 1.2020569\dots$ ,  $z4 = \zeta_4 = 1.0823232\dots$ ,  $z5 = \zeta_5 = 1.0369278\dots$ .  
`cf` =  $C_F$  and `ca` =  $C_A$  are the quadratic Casimir operators of the quark  $[T^a T^a]_{ij} = C_F \delta_{ij}$  and the adjoint  $[C^a C^a]_{bd} = C_A \delta_{bd}$ ,  $(C^a)_{bc} = -if^{abc}$  representations of the Lie algebra, `ng` and `dR` are dimensions of the adjoint (gluon) and quark representations of the gauge group, `nf` stands for the number of quark flavors and `tr` =  $T_f$  refers to the trace normalization  $\text{tr}(T^a T^b) = T_f \delta^{ab}$ .

Anc1.mres:

File `Anc1.mres` defines three functions `Dgg[k,m,1]`, `Dqg[k,m,1]`, `Dqq[k,m,1]`. Their relation to the function

$$(D_\ell)_{km}^{\alpha\beta}$$

as defined in eq. (44) of the paper is as follows:

$$(D_\ell)_{km}^{gg} = \text{Dgg}[k, m, \ell] G_0^\ell, \tag{1}$$

$$(D_\ell)_{km}^{qg} = \text{Dqg}[k, m, \ell] G_0^\ell, \tag{2}$$

$$(D_\ell)_{km}^{qq} = \text{Dqq}[k, m, \ell] G_0^\ell, \tag{3}$$

where

$$G_0 = \frac{\Gamma(1 + \epsilon)\Gamma(1 - \epsilon)^2}{\Gamma(2 - 2\epsilon)}. \tag{4}$$

A choice of the prefactor  $G_0$  fixes a particular version of a minimal scheme<sup>1</sup>. Eq. (4) corresponds to the standard MS-scheme [1] while two other popular minimal schemes  $\overline{\text{MS}}$ -one [2] and the G-scheme [3] are fixed by the choice:

$$G_0^{\overline{\text{MS}}} = G_0 e^{\gamma_E} \quad \text{and} \quad G_0^G = 1, \tag{5}$$

with  $\gamma_E = 0.577216\dots$ , being the Euler constant appearing in the expansion of the Gamma function

$$\Gamma(1 + \epsilon) = 1 - \gamma_E \epsilon + \mathcal{O}(\epsilon^2).$$

Note also that the functions  $D_{\alpha\beta}[k, m, \ell]$  are presented as series in  $\epsilon$ . The maximal power of  $\epsilon$  corresponds to  $\epsilon^2$ ,  $\epsilon^1$  and  $\epsilon^0$  for  $\ell = 1, 2$  and  $3$  correspondingly. In addition, the function `Dqq[k, m, ℓ]` is internally decomposed in two pieces, namely, the singlet and nonsinglet ones with the help of two auxiliary labels `si` and `ns`. Before using the results from file `Anc1.mres` for construction off-diagonal anomalous dimensions one should first set `si` = `ns` = 1.

Anc2.mres:

File `Anc2.mres` contains our results for the anomalous dimensions matrix in Eq. (33) and the matrix `B` defined in Eq. (40). In all expressions in this file the trace normalization factor `tr` is set to its canonical value 1/2.

---

<sup>1</sup>We assume that all Z-factors are to be chosen as containing only poles in  $\epsilon$  (not counting the leading 1).

The  $8 \times 8$  matrices `gammaOffdiag2loop` and `gammaOffdiag3loop` contain off-diagonal blocks of the matrix in Eq. (33) at two loops and three loops, respectively. The results presented in Eqs. (57)–(61) correspond to the  $2 \times 2$  blocks of this matrix for the QCD case  $C_A = 4/3$ ,  $C_F = 4/3$ .

The  $8 \times 8$  matrices `gammaDiag1loop`, `gammaDiag2loop` and `gammaDiag3loop` contain the block-diagonal parts (one loop, two loops and three loops) of the anomalous dimension matrix  $\widehat{\gamma}_n(a)$  defined in Eq.(35). The  $2 \times 2$  blocks in these matrices are also given in `gammakl`, where  $k = 1, 3, 5, 7$  stands for the number of derivatives in the quark operator (spin  $N = k + 1$ ) and  $l = 1, 2, 3$  is the number of loops.

The  $8 \times 8$  matrices `B1loop`, `B2loop` contain one-loop  $O(a)$  and two-loop  $O(a^2)$  contributions to the matrix  $\mathbf{B}$  defined in Eq. (40).

- [1] G.'t Hooft, Nuclear Physics B 61, 455 (1973).
- [2] W.A. Bardeen, A.J. Buras, D.W. Duke, T. Muta, Physical Review D. 18 (11): 3998–4017 (1978).
- [3] K. G. Chetyrkin, A. L. Kataev and F. V. Tkachov, Nucl. Phys. B **174**, 345, (1980).
